# Supplementary material for: Genetic redundancies enhance information transfer in noisy regulatory circuits
Source: arXiv:1602.07082 source file (2016-02-23)

# Supplementary Material

# Methods

## Model of a simple regulated system

As a simple regulatory model, we considered a redundant system consisting of $N$ different transcriptional units each of them activated by the input signal ($x$). The model for the $i$-th unit reads

$$\frac{dy_i}{dt} = \alpha_0 + \frac{\alpha x(t)^n}{1 + x(t)^n} - y_i + q_i(y_i, x)\xi_i(t), \tag{1}$$

where expression and time are appropriately rescaled to have a dimensionless model. The parameter values are $\alpha_0 = 0.01$, $\alpha = 2.5$, and $n = 2$. In addition, the statistics of $\xi_i$ are $\langle \xi_i(t) \rangle = 0$ and $\langle \xi_i(t_0)\xi_i(t_0 + t) \rangle = \delta(t)$. Noise amplitude is given by $q_i(y_i, x) = \sqrt{\frac{1}{K}\left(\alpha_0 + \frac{\alpha x^n}{1 + x^n} + y_i\right)}$. The parameter $K$ is proportional to the effective dissociation constant between the transcription factor and the promoter, and determines the number of molecules of the system and then intrinsic noise [1]. Otherwise specified, we considered $K = 100$.

## Model of a bistable system

We considered that each of the $N$ units of the system is a gene activating transcriptionally its own expression. This corresponds to a minimal implementation of a bistable system. The model for the $i$-th unit reads

$$\frac{dy_i}{dt} = \alpha_0 + \frac{\alpha y_i^n}{1 + y_i^n} - y_i + x(t) + q_i(y_i)\xi_i(t), \tag{2}$$

where expression and time are appropriately rescaled to have a dimensionless model. Now, the input signal ($x$) is introduced as a small perturbation. The parameter values are the same as before, as well as the statistics of $\xi_i$. Noise amplitude is given by $q_i(y_i) = \sqrt{\frac{1}{K}\left(\alpha_0 + \frac{\alpha y_i^n}{1 + y_i^n} + y_i\right)}$, having neglected the effect of $x$.

To account for extrinsic noise, we introduced a new stochastic process ($\xi_{ex}$), common to all units, in Eq. (2) as

$$\frac{dy_i}{dt} = \alpha_0 + \frac{\alpha y_i^n}{1 + y_i^n} - y_i + x(t) + q_i(y_i)\xi_i(t) + q_{ex}\xi_{ex}(t). \tag{3}$$

The correlation time of extrinsic noise is of the order of the cell cycle [2] (the mean is also 0). For simplicity, we here considered a system implemented with short-lived proteins, so we can assume that $\xi_{ex}$ is constant within the time window that the system needs to reach its steady state upon receiving the perturbation $x$.

To account for heterogeneity in the different units of the system, we followed

$$\frac{dy_i}{dt} = \alpha_0 + \frac{\alpha (\omega_i y_i)^n}{1 + (\omega_i y_i)^n} - y_i + x(t) + q_i(y_i)\xi_i(t), \tag{4}$$

where the standard deviation of $\omega_i$ (a Gaussian random number with mean 1) quantifies the degree of heterogeneity.

To account for certain cross-talk between the different units of the system, we followed a perturbative approach on Eq. (2) to obtain

$$\frac{dy_i}{dt} = \alpha_0 + \frac{\alpha y_i^n}{1 + y_i^n} - y_i + x(t) + q_i(y_i)\xi_i(t) + \varepsilon \sum_{j=1, j\neq i}^{N} y_j, \tag{5}$$

where $\varepsilon$ quantifies the degree of cross-talk. For simplicity, we assumed $q_i(y_i)$ not to be dependent on $y_j$ for $j \neq i$.

## Model of an excitable system

We considered the model proposed to explain competence in *Bacillus subtilis*, associated with the capability for DNA uptake from the environment, by which the cell can reach transient differentiation [3]. Each of the $N$ units of the system consists of two transcriptional units ($y_i$ and $z_i$) that implement, in an effective way, interlinked positive and negative feedback loops. The model for the $i$-th unit reads

$$\begin{aligned} \frac{dy_i}{dt} &= \alpha_0 + \frac{\alpha\,(\sigma y_i)^n}{1+(\sigma y_i)^n} - \frac{y_i}{1+y_i+z_i}, \\ \frac{dz_i}{dt} &= \frac{\beta}{1+(\sigma y_i)^m} - \frac{z_i}{1+y_i+z_i} + x(t) + q\xi_i(t), \end{aligned} \tag{6}$$

where expression and time are appropriately rescaled to have a dimensionless model. The parameter values are $\alpha_0 = 0.004$, $\alpha = 0.07$, $\beta = 0.826$, $\sigma = 5$, $n = 2$, and $m = 5$. Here, noise amplitude is approached as a constant ($q = \sqrt{(\beta+1)/K}$, with $K = 500$), and $\xi_i$ follows the same statistics as before.

## Input and output variables

The input signal ($x$) is a random number given by $x = \langle x\rangle 10^u$, where $u$ corresponds to a random number uniformly distributed in $[-1, +1]$, unless otherwise specified. In case of the simple regulated system, we took $\langle x\rangle = 1$; in case of the bistable system, $\langle x\rangle = 0.001$ in Fig. 2, and $\langle x\rangle = 0.005$ in Figs. 4-5; and in case of the excitable system, $\langle x\rangle = 0.9$. We considered $\log x$ as input variable to compute information transfer. In addition, $x$ is a step function (at $t = 0$) in case of the simple regulated and bistable systems, and a pulse function for one unit of normalized time (at $t = 0$) in case of the excitable device.

As output, we established the steady state of the system response upon induction with the input signal. Initially ($t = 0$), we assumed $x = 0$. Thus, we defined $\Delta y_i = y_i(x) - y_i(x = 0)$. The total differential gene expression of the redundant system can be written as $\Delta y = \sum_{i=1}^{N} \Delta y_i$. In case of the excitable system, because the response is transient, we considered a Boolean function operating on $y_i$, setting 1 if the unit was excited or 0 if not.

## Calculation of mutual information

To calculate mutual information, we solved numerically the following integral

$$I = -\int_{-\infty}^{+\infty} P_{\Delta y}(s)\log_2 P_{\Delta y}(s)ds + \int_{-\infty}^{+\infty} P_{\log x}(r)\int_{-\infty}^{+\infty} P_{\Delta y|\log x}(s)\log_2 P_{\Delta y|\log x}(s)dsdr, \tag{7}$$

where we considered $\log x$ as input and $\Delta y$ as output variables.

By using the Fokker-Planck equation, we calculated the probability that a unit has a given expression level, $P_i(y_i|x)$ [4]. The effective stochastic potential ($\phi_i$) associated to Eq. (2) [and also to Eq. (1)] is

$$\phi_i(y_i, x) = -\int_0^{y_i} \frac{f_i(s,x)}{q_i(s)^2}ds + \log q_i(y_i), \tag{8}$$

having defined $f_i$ as the right-hand side (without the stochastic process). Thus, $P_i(y_i|x) = Ce^{-2\phi_i(y_i,x)}$, where $C$ is a normalization constant so that $\int_0^{\infty} P_i(s|x)ds = 1$. In addition, when considering extrinsic noise (for the bistable system), we got

$$\phi(y_i, x) = -\int_0^{y_i} \frac{f_i(s, x+\zeta)}{q_i(s)^2}ds + \log q_i(y_i), \tag{9}$$

where $\zeta$ is a Gaussian random number with mean 0 and standard deviation $q_{ex}$. In case of cross-talk, we got

$$\phi_i(y_1, y_2, ..., y_N, x) = -\int_0^{y_i} \frac{f_i(s,x)}{q_i(s)^2}ds + \log q_i(y_i) - \varepsilon \sum_{j=1, j\neq i}^{N} y_j \int_0^{y_i} \frac{1}{q_i(s)^2}ds. \tag{10}$$

In case of the excitable system, we calculated $P_i(y_i, z_i|x)$ numerically.

### Calculation of distance to linear response

To calculate distance to linear response ($d_{lin}$) [5], we averaged all realizations of $y_i$ for a given $x$ to obtain an average response ($\langle \Delta y_i(x) \rangle$, taking into account the initial conditions). Note that $x$ varies uniformly between $x_{min}$ and $x_{max}$. In case of the bistable system, the two output values in the deterministic regime are approximately $\alpha_0$ and $(\alpha + \sqrt{\alpha^2 - 4})/2$. Then, we considered the ideal linear response as $y_{lin} = \alpha_0 + \frac{\alpha + \sqrt{\alpha^2 - 4}}{2} \frac{x - x_{min}}{x_{max} - x_{min}}$. And the calculation of the distance reads

$$d_{lin,i} = \int_{x_{min}}^{x_{max}} \left( \langle \Delta y_i(x) \rangle - y_{lin}(x) \right)^2 dx. \tag{11}$$

## References

[1] Rodrigo G, Kirov B, Shen S, Jaramillo A (2013) Theoretical and experimental analysis of the forced LacI-AraC oscillator with a minimal gene regulatory model. *Chaos* 23: 025109.

[2] Rosenfeld N, Young JW, Alon U, Swain PS, Elowitz MB (2005) Gene regulation at the single-cell level. *Science* 307: 1962-1965.

[3] Süel G, Garcia-Ojalvo J, Liberman L, Elowitz MB (2006) An excitable gene regulatory circuit induces transient cellular differentiation. *Nature* 440: 545-550.

[4] Frigola D, Casanellas L, Sancho JM, Ibañes M (2012) Asymmetric stochastic switching driven by intrinsic molecular noise. *PLoS One* 7: e31407.

[5] Gammaitoni L (1995) Stochastic resonance and the dithering effect in threshold physical systems. *Phys Rev E* 52: 4691-4698.

# Supplementary Figures

## Figure S1

Dependence of distance of the average response to the ideal linear response with the intrinsic noise amplitude. Given the deterministic steady states of the system, we computed the ideal linear response; $y$, the gene expression level of the device (and then $\Delta y$, the difference with respect to the initial state), as a function of $x$, the magnitude of the signal. This plot corresponds to the bistable unit ($N = 1$). It shows a minimum in distance for certain amount of noise. Here, the distribution of the input signal values is a uniform with a mean of 0.005 and a variance that allows covering two orders of magnitude. Distributions of $\Delta y$ versus $x$ are shown for different points. They display the responses of the device to $10^4$ signal values drawn from the described distribution (black dots). The real average response of the system (averaging all possible responses $\Delta y$ due to noise for a given value of $x$) together with the ideal linear response are shown.

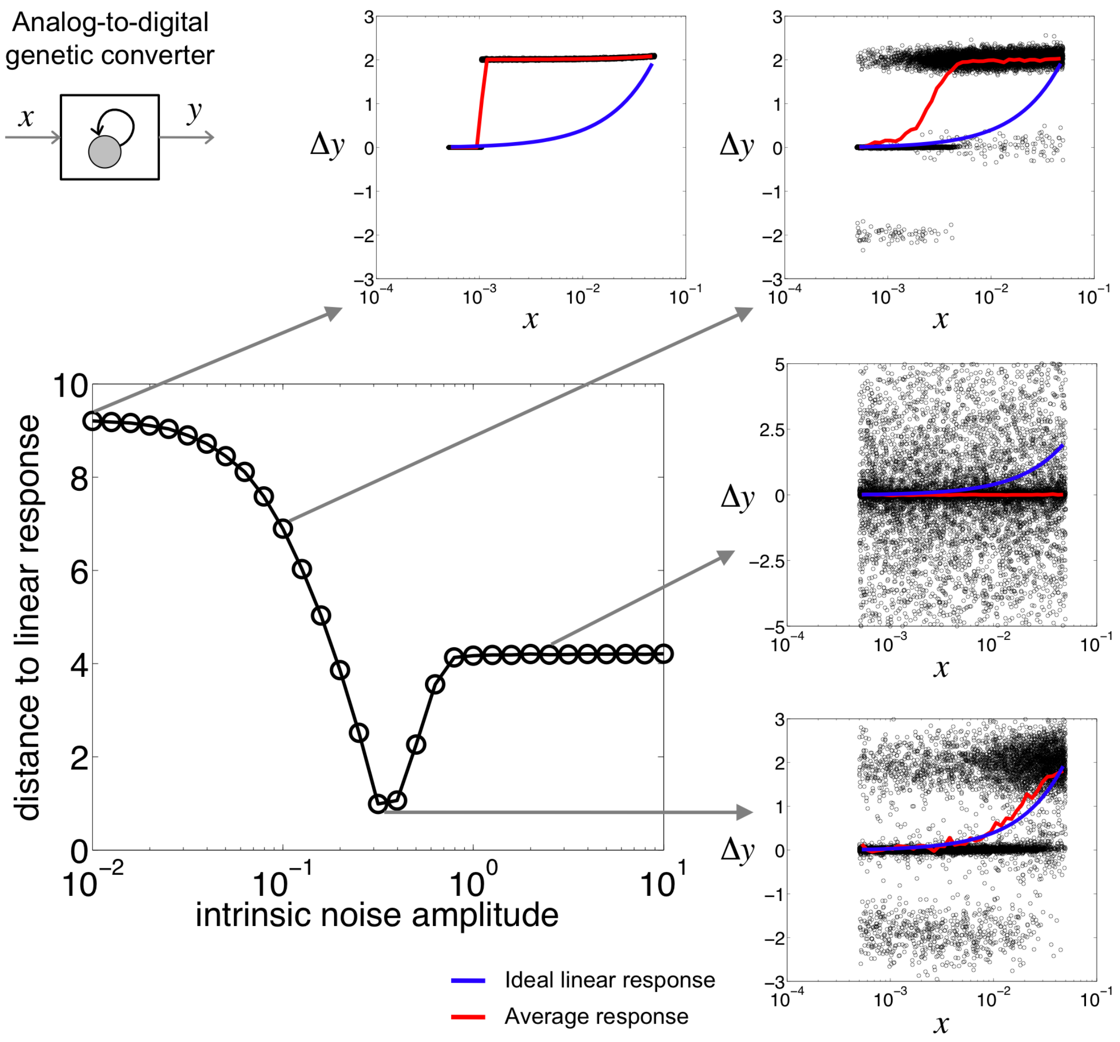

## Figure S2

(A) Dependence of mutual information with the feedback strength (or also intrinsic noise amplitude, parameterized by $1/K$) of the bistable unit. The inset shows the effective stochastic potential ($\phi$) for $K = 100$ and $K = 1000$ (with $N = 2$). Certainly, it shows two potential wells (i.e., two stable steady states), and the threshold of the system is within (note that intrinsic noise is multiplicative, i.e., the amplitude of the stochastic fluctuations depends on the particular gene expression level). In case of higher noise ($K = 100$), the potential barrier is very low, indicating that it is very easy to have stochastic threshold crossings. However, in case of lower noise ($K = 1000$), the potential barrier is high, moderating the number of stochastic threshold crossings. The observed trend of information transfer versus intrinsic noise (higher the noise, higher the information transfer) is explained because the stochastic threshold crossings (for a continuous output variable, and to some extent) is the mechanism underlying the linearization of the response and the increase of communication fidelity. (B) Dependence of mutual information with the number of units ($N$) of the system. Relative mutual information is with respect to $N = 1$ for different intrinsic noise levels (modulated by $K$). This shows how the higher the intrinsic noise level, the stronger the amplification of information transfer due to genetic redundancy.

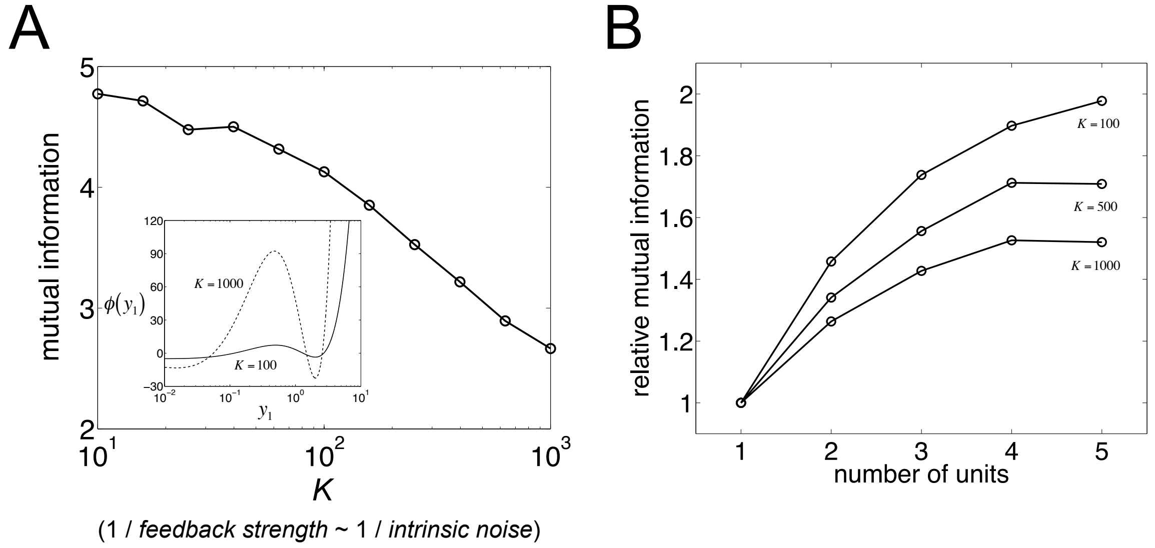

## Figure S3

Dependence of mutual information with the number of units ($N$) for an excitable system. On top, input/output distributions depicting information transfer. The input distribution (in yellow) is assumed to be uniform (with a mean of 0.9 and a variance that allows covering two orders of magnitude). Output distributions (in gray) illustrate the processing of the signal $x$, either through a single copy of the threshold device (left) or an array of multiple redundant copies (right). Note that the output is Boolean, setting if the unit is excited or 0 if not. In the latter case, each unit of the array receives the same signal and the output $y$ is the sum of all the individual responses. Redundancy effectively enlarges the alphabet of the response. This is reflected in the output distribution, and also in the linearization of the averaged stimulus-response profile (black curve). On bottom, relative mutual information is with respect to $N = 1$. For this plot, we considered a system of $N$ excitable units implemented with interlinked positive and negative feedbacks. According to the same input level, each unit can decide, in presence of molecular noise, to either perform an excursion over the phase space (excitation) or not. The inset shows the phase space where the nullclines (black lines) determine the possible trajectories of the system (gray lines, deterministic regime). The arrows indicate direction. The point corresponds to the stable steady state. Note that a perturbation (in gene $z$) provokes the excitation of the system provided its magnitude ($x$) is large enough, otherwise the system falls down to the steady state as it is within the basin of attraction.

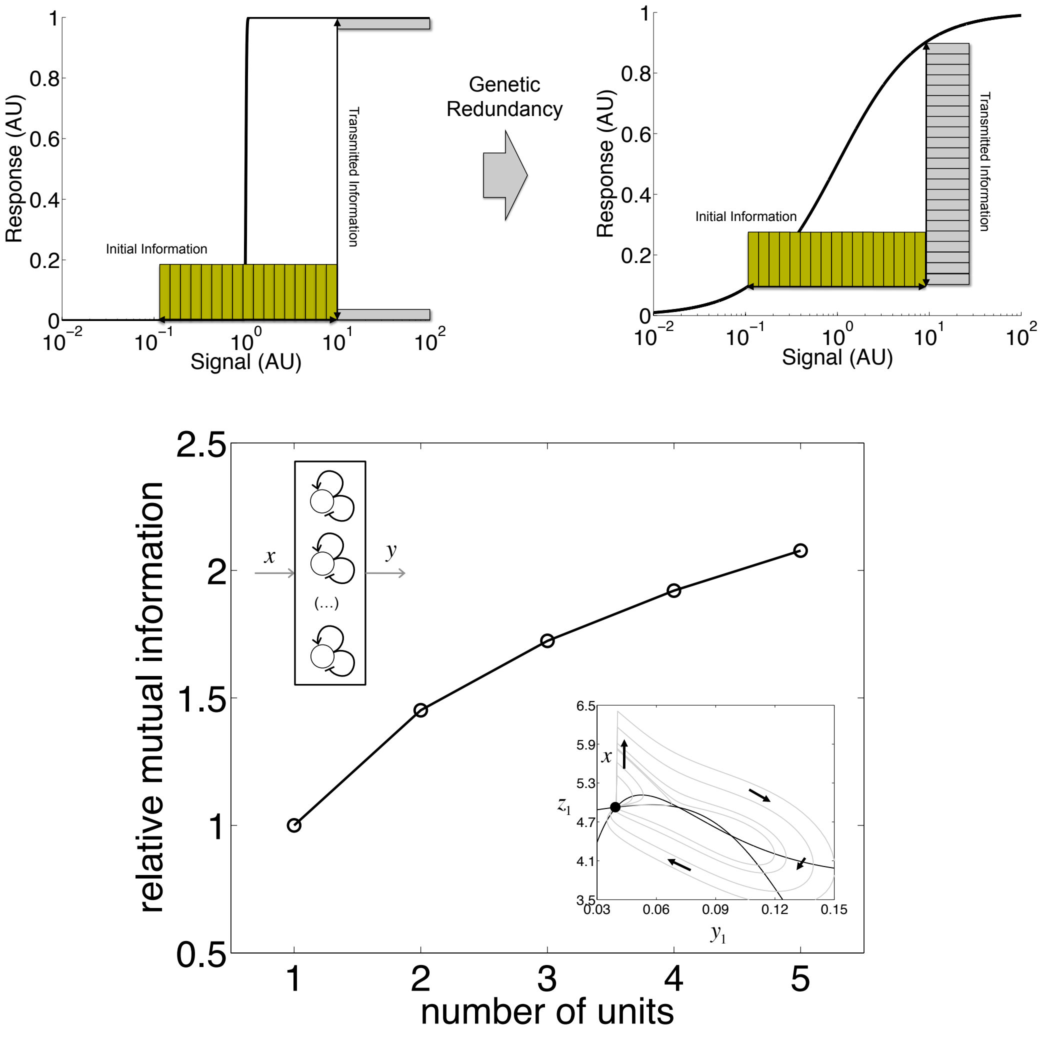

Supplement: Supplementary file 1 [file Supplement.pdf]
